# Supplementary material for: Understanding magnetoelectric switching in BiFeO$_3$ thin films
Source: arXiv:2307.14789 ancillary file (2023-07-27)
Supplement: Supplementary file 1 [file supplementary.pdf]

# Understanding magnetoelectric switching in $BiFeO_3$ thin films
# - Supplementary Material -

Natalya S. Fedorova,[1,*] Dmitri E. Nikonov,[2] John M. Mangeri,[1] Hai Li,[2] Ian A. Young,[2] and Jorge Íñiguez[1,3,†]

[1]*Materials Research and Technology Department, Luxembourg Institute of Science and Technology, 5 Avenue des Hauts-Fourneaux, L-4362 Esch/Alzette, Luxembourg*

[2]*Components Research, Intel Corporation, Hillsboro, 97124 Oregon, USA*

[3]*Department of Physics and Materials Science, University of Luxembourg, 41 Rue du Brill, L-4422 Belvaux, Luxembourg*

## SI. DOMAIN WALL ENERGY DUE TO STRUCTURAL DISCONTINUITY

In this section, we describe how we give an estimate for the parameters $K_{DW,P}$ and $K_{DW,R}$ of the $F_{DW,P}$ and $F_{DW,R}$ terms (Eqs. (13) and (14) of the main text), respectively, using the energies of the neutral domain walls (DWs) computed for $BiFeO_3$ by Dieguez *et al.*[1].

As it has been demonstrated in the aforementioned work, the largest contribution to the DW energy originates from the discontinuity in the $FeO_6$ octahedral tilts **R**. To take this into account, we consider (110) 180° DW (all components of **P** and **R** change their signs at the wall) with the energy per unit area (ua) of $F_{DW,ua} = 255$ mJ m$^{-2}$, and separate it to two contributions: $F_{DW,P,ua} = 1/3 F_{DW,ua} = 85$ mJ m$^{-2}$ and $F_{DW,R,ua} = 2/3 F_{DW,ua} = 170$ mJ m$^{-2}$. These fractions are selected based on the fact that the energy of the (110) DW in $BiFeO_3$ at which all components of **P** are reversed while **R** remains unaffected is nearly 1/3 of the energy of the DW at which both **P** and **R** are reversed, see Ref. 1 for the details.

Next, we write an expression for $F_{DW,P,ua}$ using Eq. (13) of the main text for the system of two domains (with open boundary conditions) having opposite $\mathbf{P}_i$ :

$$F_{DW,P,ua} = \frac{1}{2} K_{DW,P}[(P_{1,x} - P_{2,x})^2 + (P_{1,y} - P_{2,y})^2 + (P_{1,z} - P_{2,z})^2], \tag{S1}$$

where $\mathbf{P}_1$ and $\mathbf{P}_2$ are the polarizations of the domains #1 and #2. Since $P_1 = -P_2$ and $|P_{i,x}| = |P_{i,y}| = |P_{i,z}|$, we can simplify this expression to:

$$F_{DW,P,ua} = 6K_{DW,P}(P_{1,x})^2. \tag{S2}$$

Therefore,

$$K_{DW,P} = \frac{F_{DW,P,ua}}{6(P_{1,x})^2}. \tag{S3}$$

According to our previous work[2], $P_x = 0.546$ C m$^{-2}$, hence:

$$K_{DW,P} = \frac{F_{DW,P,ua}}{6(P_{1,x})^2} = 0.0476 \text{ J m}^2 \text{ C}^{-2}. \tag{S4}$$

Similarly, we can write the energy $F_{DW,R,ua}$ (per unit area) of the system of two domains with opposite **R**:

$$F_{DW,R,ua} = \frac{1}{2} K_{DW,R}[(R_{1,x} - R_{2,x})^2 + (R_{1,y} - R_{2,y})^2 + (R_{1,z} - R_{2,z})^2], \tag{S5}$$

from which we obtain:

$$K_{DW,R} = \frac{E_{DW,R}}{6(R_{1,x})^2}. \tag{S6}$$

Using the value $R_x = 7.737$ deg from Ref. 2, we obtain $K_{R,DW} = 4.73 \times 10^{-4}$ J m$^{-2}$ deg$^{-2}$.

## SII. POLARIZATION SWITCHING IN MONODOMAIN $BiFeO_3$

Table S1. Statistics of polarization switching events in the simulations of monodomain bulk $BiFeO_3$ at T=300 K with no applied electric field. $Q_P$ (in F $m^{-1}$ $s^{-1}$) and $Q_R$ (in $\times 10^4$ $deg^2$ $m^3$ $J^{-1}$ $s^{-1}$) define the noise amplitudes for **P** and **R**, respectively. $M$ is the number of the simulations (in % out of 200 runs) in which **P** and **R** did not switch any of their components. The last row of the table shows the statistic for the default values of $Q_P = L_P$ and $Q_R = L_R$.

| $Q_P$ | $Q_R$ | $M$ |
|---|---|---|
| 120 | 5.00 | 100.0 |
| | 6.00 | 99.5 |
| | 7.00 | 99.5 |
| | 8.00 | 96.0 |
| 140 | 5.00 | 99.0 |
| | 6.00 | 96 |
| | 7.00 | 94.5 |
| | 8.00 | 89 |
| 160 | 5.00 | 98.5 |
| | 6.00 | 91 |
| | 7.00 | 81.5 |
| | 8.00 | 66 |
| 180 | 5.00 | 87.5 |
| | 6.00 | 78 |
| | 7.00 | 65 |
| 200 | 8.32 | 9.5 |

Table S2. Statistics of polarization switching events in the simulations of monodomain bulk $BiFeO_3$ at T=300 K under the applied electric field with the amplitude $E_{max}$. $Q_P$ (in F $m^{-1}$ $s^{-1}$) and $Q_R$ (in $\times 10^4$ $deg^2$ $m^3$ $J^{-1}$ $s^{-1}$) define the noise amplitudes for **P** and **R**, respectively. $M_0$ is the number of the simulations in which **P** and **R** did not switch any of their components; $M_1$ denotes the number of simulations in which **P** and **R** switched only once their $z$ component; $M_{other}$ is the number of simulations in which **P** and **R** switched more than once. $M_0$, $M_1$ and $M_{other}$ are given in % out of 200 runs.

| $Q_P$ | $Q_R$ | $M_0$ | $M_1$ | $M_{other}$ |
|---|---|---|---|---|
| | | $E_{max}$ = 100 MV/m | | |
| 120 | 5.00 | 98.5 | 1.5 | 0.0 |
| | 6.00 | 97.0 | 2.5 | 0.0 |
| | 7.00 | 91.0 | 9.0 | 0.0 |
| | 8.00 | 82.0 | 17.0 | 1.0 |
| 140 | 5.00 | 94.0 | 6.0 | 0.0 |
| | 6.00 | 85.5 | 12.5 | 2.0 |
| | 7.00 | 77.0 | 22.0 | 1.0 |
| 160 | 5.00 | 87.5 | 11.5 | 1.0 |
| | 6.00 | 70.5 | 26.5 | 3.0 |
| 200 | 8.32 | 0.5 | 16.5 | 83.0 |
| | | $E_{max}$ = 200 MV/m | | |
| 120 | 5.00 | 68.5 | 31.5 | 0.0 |
| | 6.00 | 43.0 | 57.0 | 0.0 |
| | 7.00 | 24.5 | 74.5 | 1.0 |
| | 8.00 | 6.5 | 90.0 | 3.5 |
| 140 | 5.00 | 34.5 | 65.5 | 0.0 |
| | 6.00 | 20.0 | 78.5 | 1.5 |
| | 7.00 | 2.5 | 92.5 | 5.0 |
| 160 | 5.00 | 9.0 | 87.0 | 4.0 |
| | 6.00 | 1.0 | 89.5 | 9.5 |

## SIII. POLARIZATION SWITCHING IN MULTIDOMAIN $BiFeO_3$ FILM

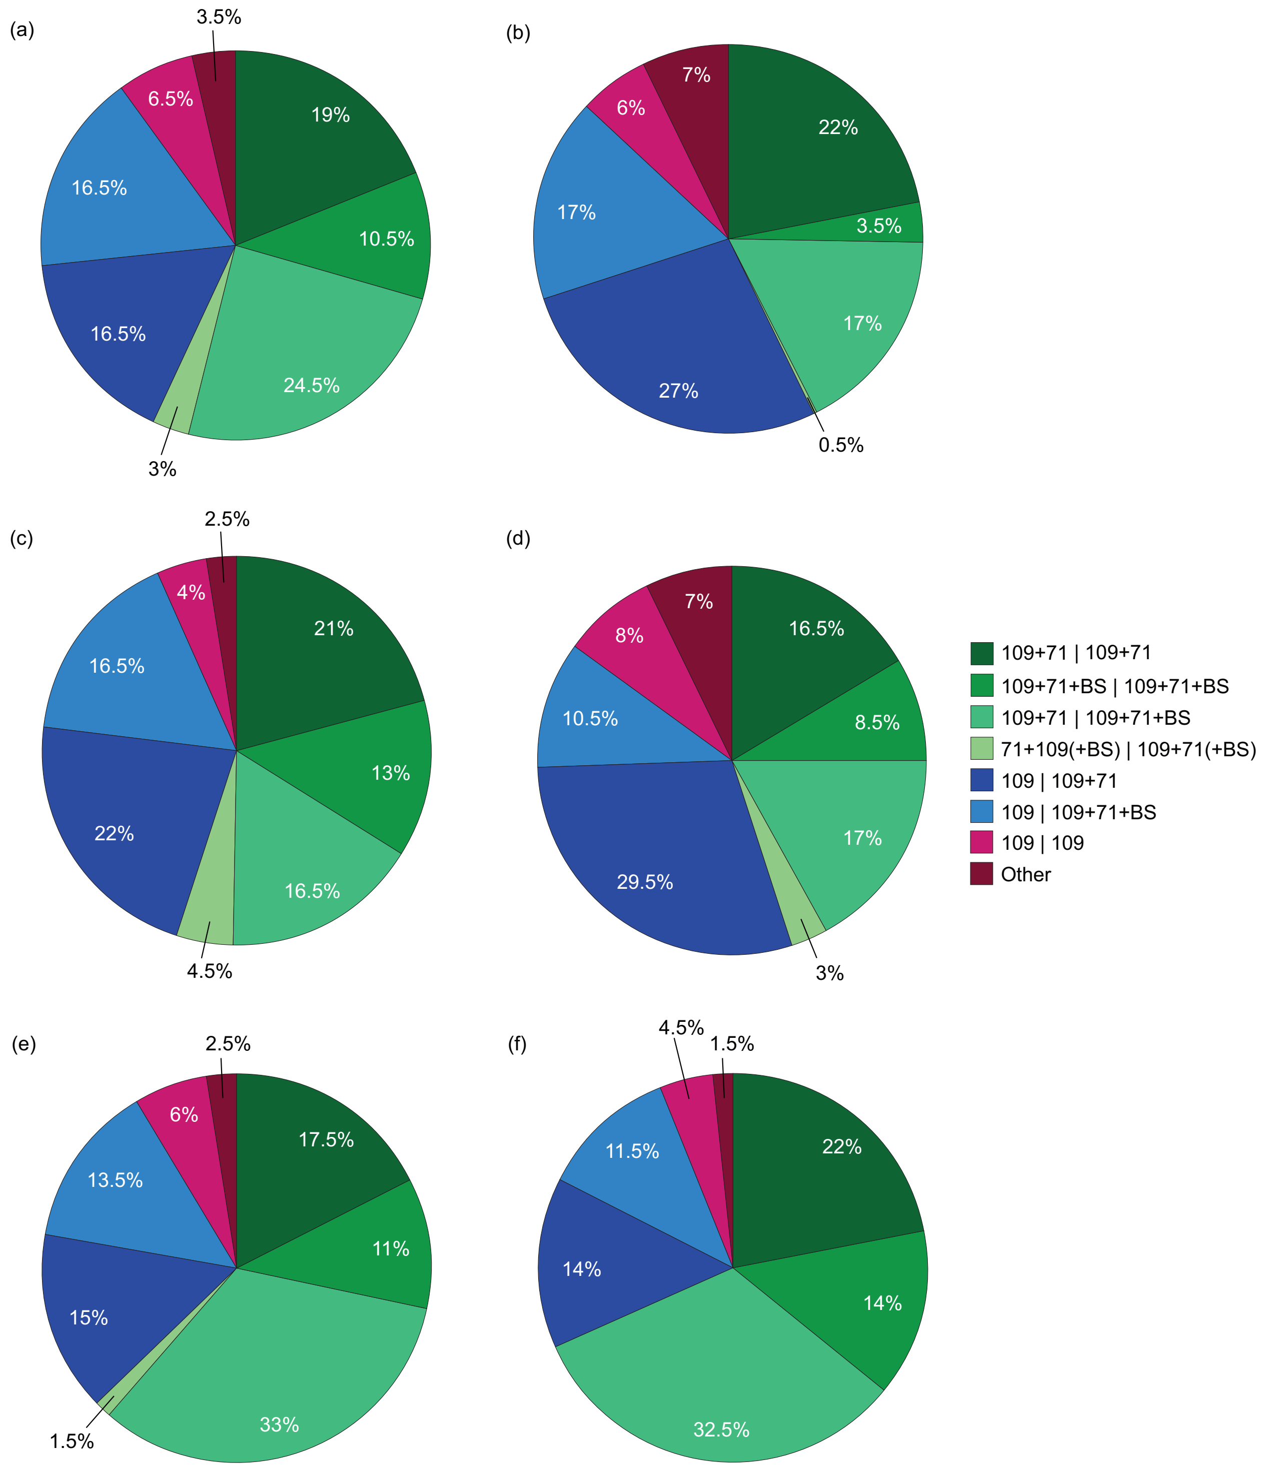


Figure S1. Statistics of polarization switching events in the dynamical simulations of multidomain $BiFeO_3$ films represented as a system of 4 domains (2 are frozen and 2 are allowed to evolve, see Fig. 4(b) of the main text) obtained using the parameter sets presented in Table II of the main text. Panel (a) shows the results obtained using the the set (i), panels (b)-(f) show the results obtained using the parameter sets (iii) - (vii). The charts shows the number of simulations (in % out of 200 runs) in which certain switching paths have been observed in two evolving domains. "BS" indicates the switching paths that involve back-and-forth switches of $P_x$. "(+BS)" indicates that the reported number includes the switching events with or without back-switches of $P_x$.

To analyze the switching behavior in the systems of more than four domains (6, 8 and 10; two domains at the ends are always frozen), we computed the number of individual domains that switched in two steps in 200 runs. For each system size, we performed this analysis using the seven parameter sets presented in Table II of the main text. As an example, let us consider the system of 6 domains among which 4 are allowed to evolve in response to the applied electric field. Since we performed 200 simulations, in each of which two domains were evolving (800 evolving domains in total), we can compute the percentage of the domains in which $\mathbf{P}_i$ reversed in $M$ number of steps with $M$ =0, 1, *etc.* The results are shown in Fig. S2. For the bigger system sizes, see Figs. S3 and S4. One can see that, in all considered cases, the high number of individual domains (more than 40%) switches in two steps.

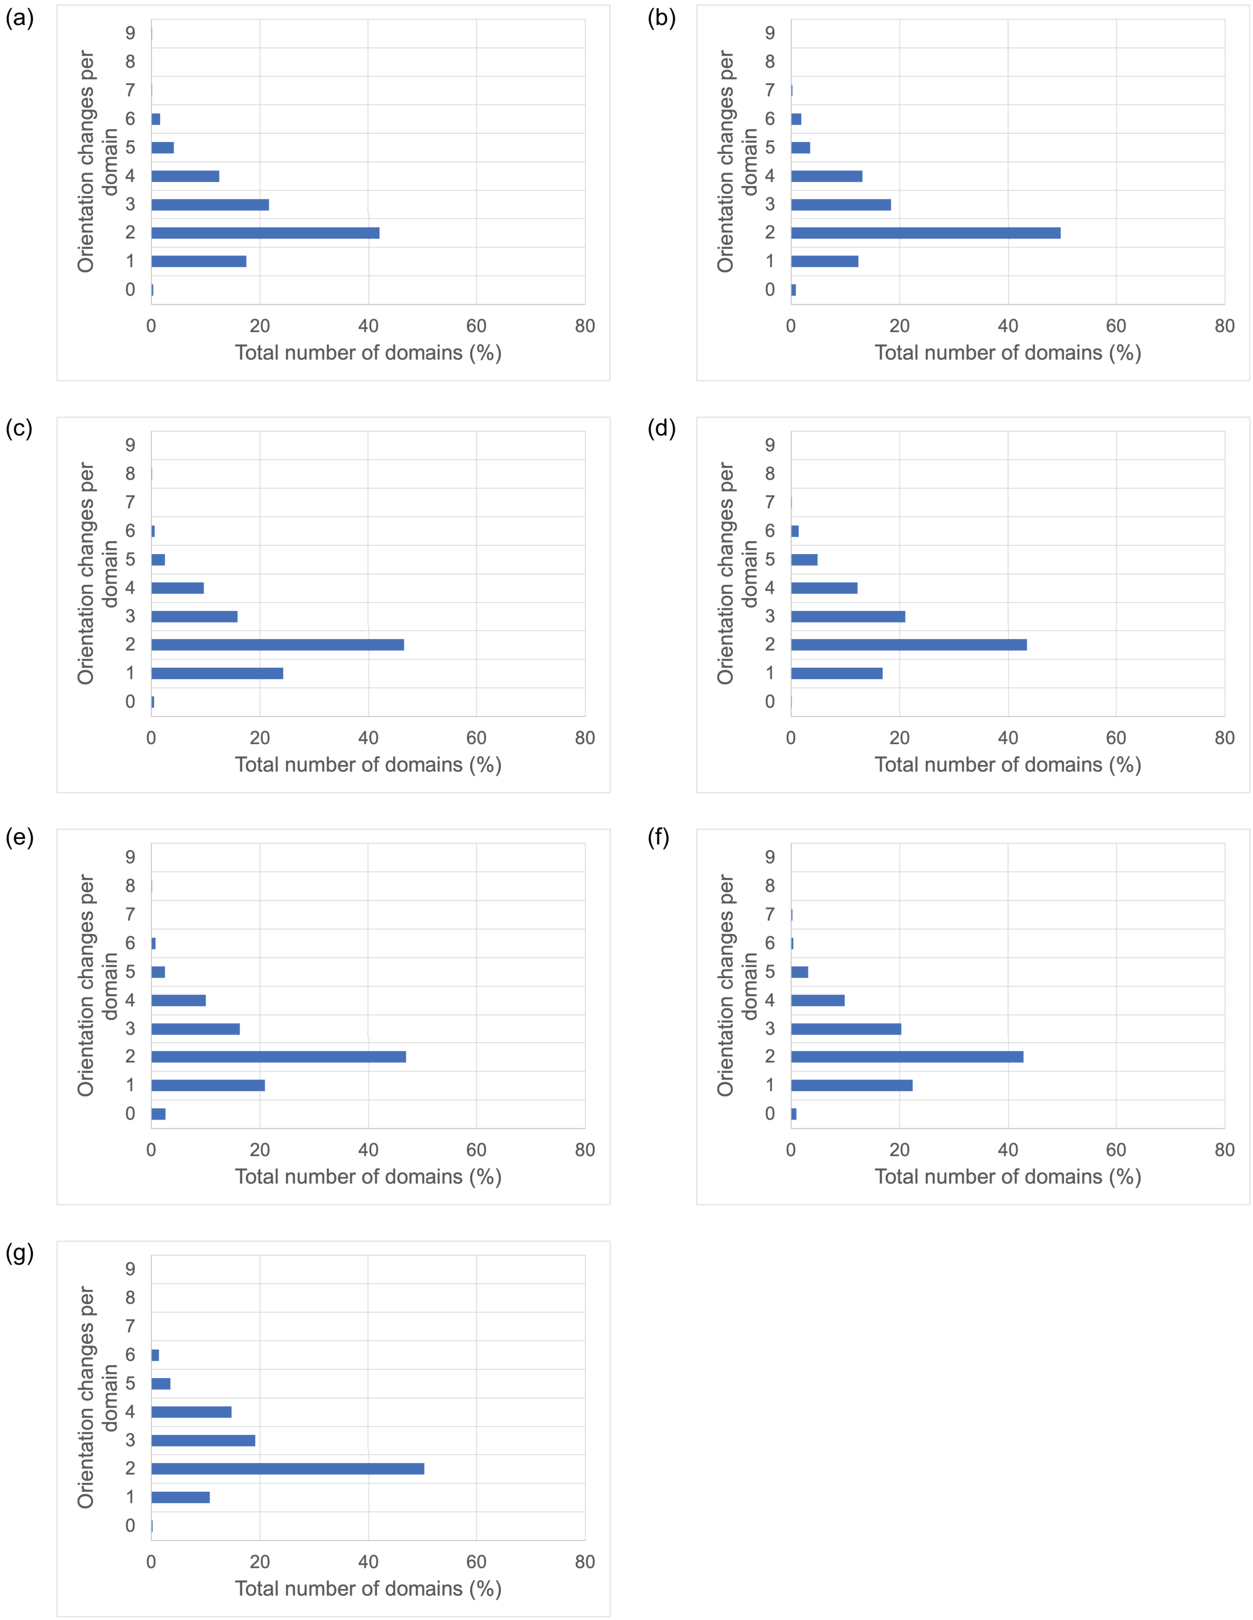


Figure S2. Statistics of polarization switching events in the dynamical simulations of multidomain $BiFeO_3$ films represented as a system of 6 domains (2 at the ends are frozen and 4 in the middle are allowed to evolve) obtained using the parameter sets presented in Table II of the main text. The histograms show the number of domains that switched in a certain number of steps in 200 runs. Panels (a) to (g) correspond to the parameter sets (i) to (vii) presented in Table II of the main text.

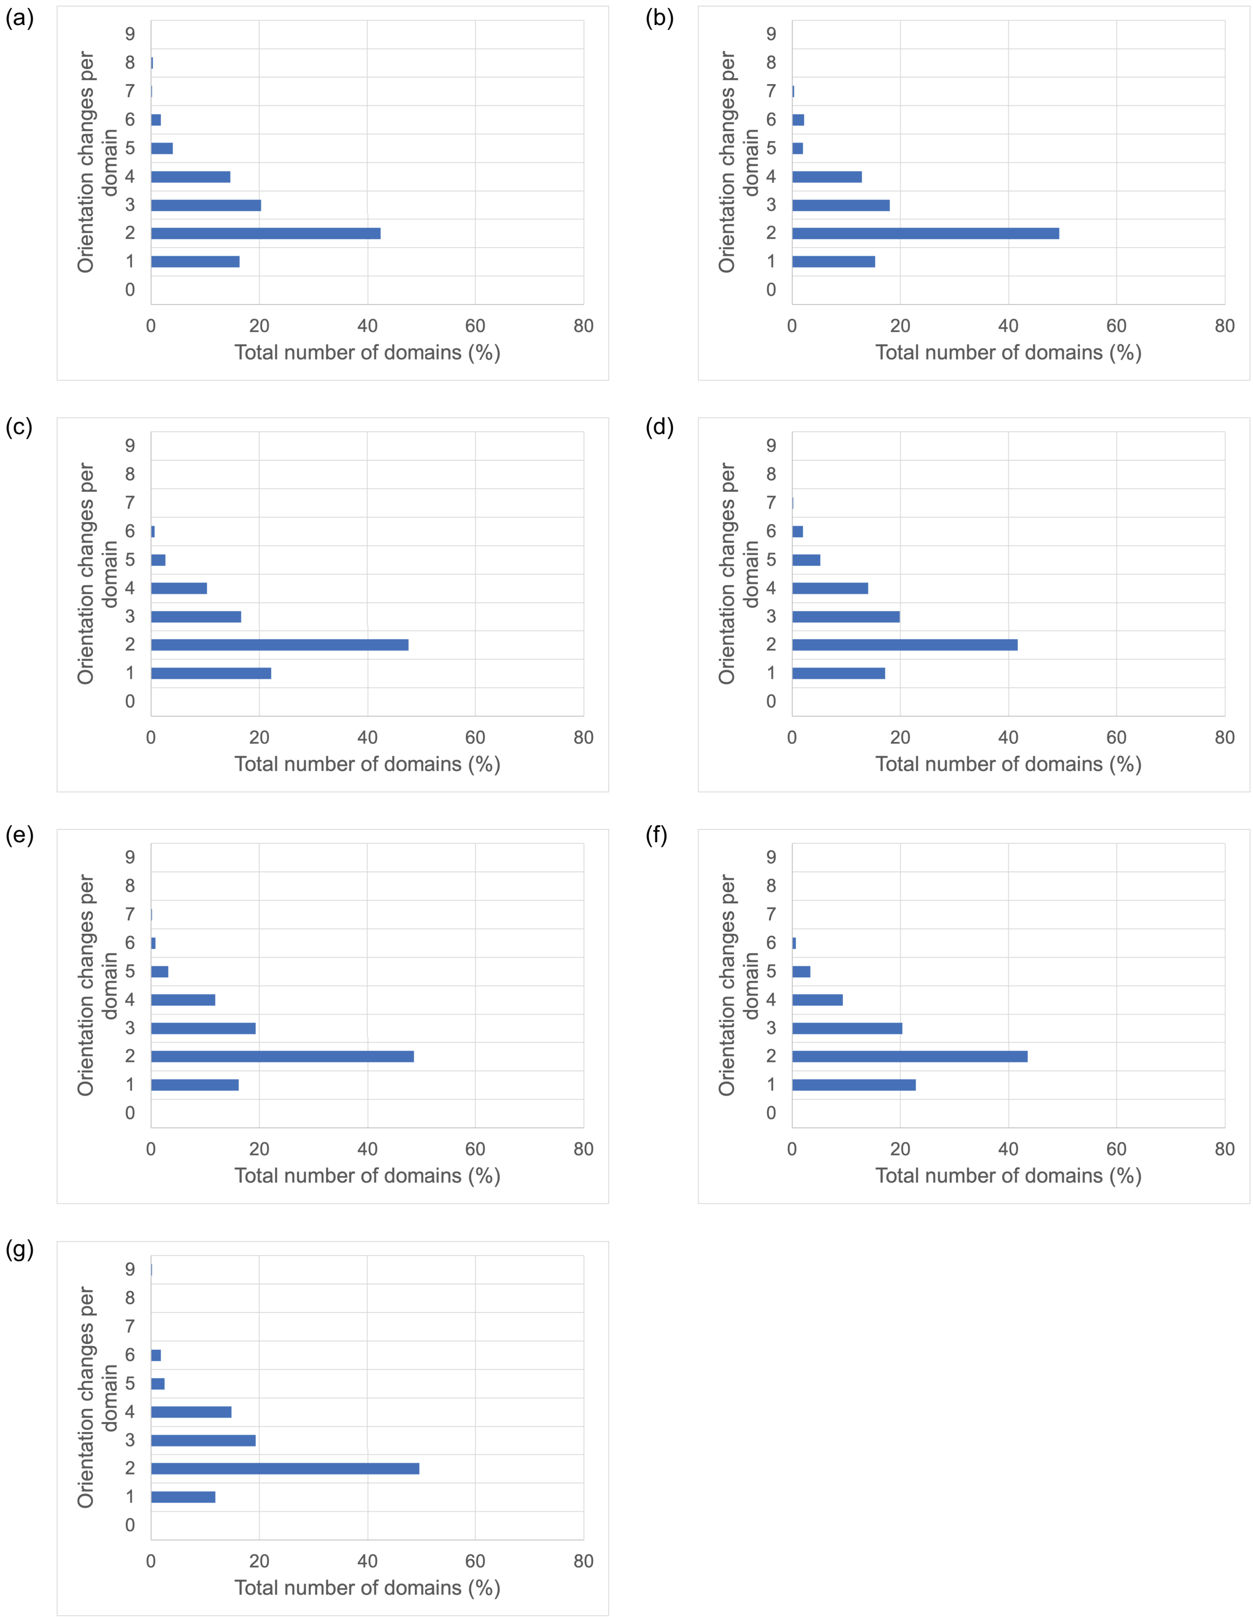


Figure S3. Statistics of polarization switching events in the dynamical simulations of multidomain $BiFeO_3$ films represented as a system of 8 domains (2 at the ends are frozen and 6 in the middle are allowed to evolve) obtained using the parameter sets presented in Table II of the main text. The histograms show the number of domains that switched in a certain number of steps in 100 runs. Panels (a) to (g) correspond to the parameter sets (i) to (vii) presented in Table II of the main text.

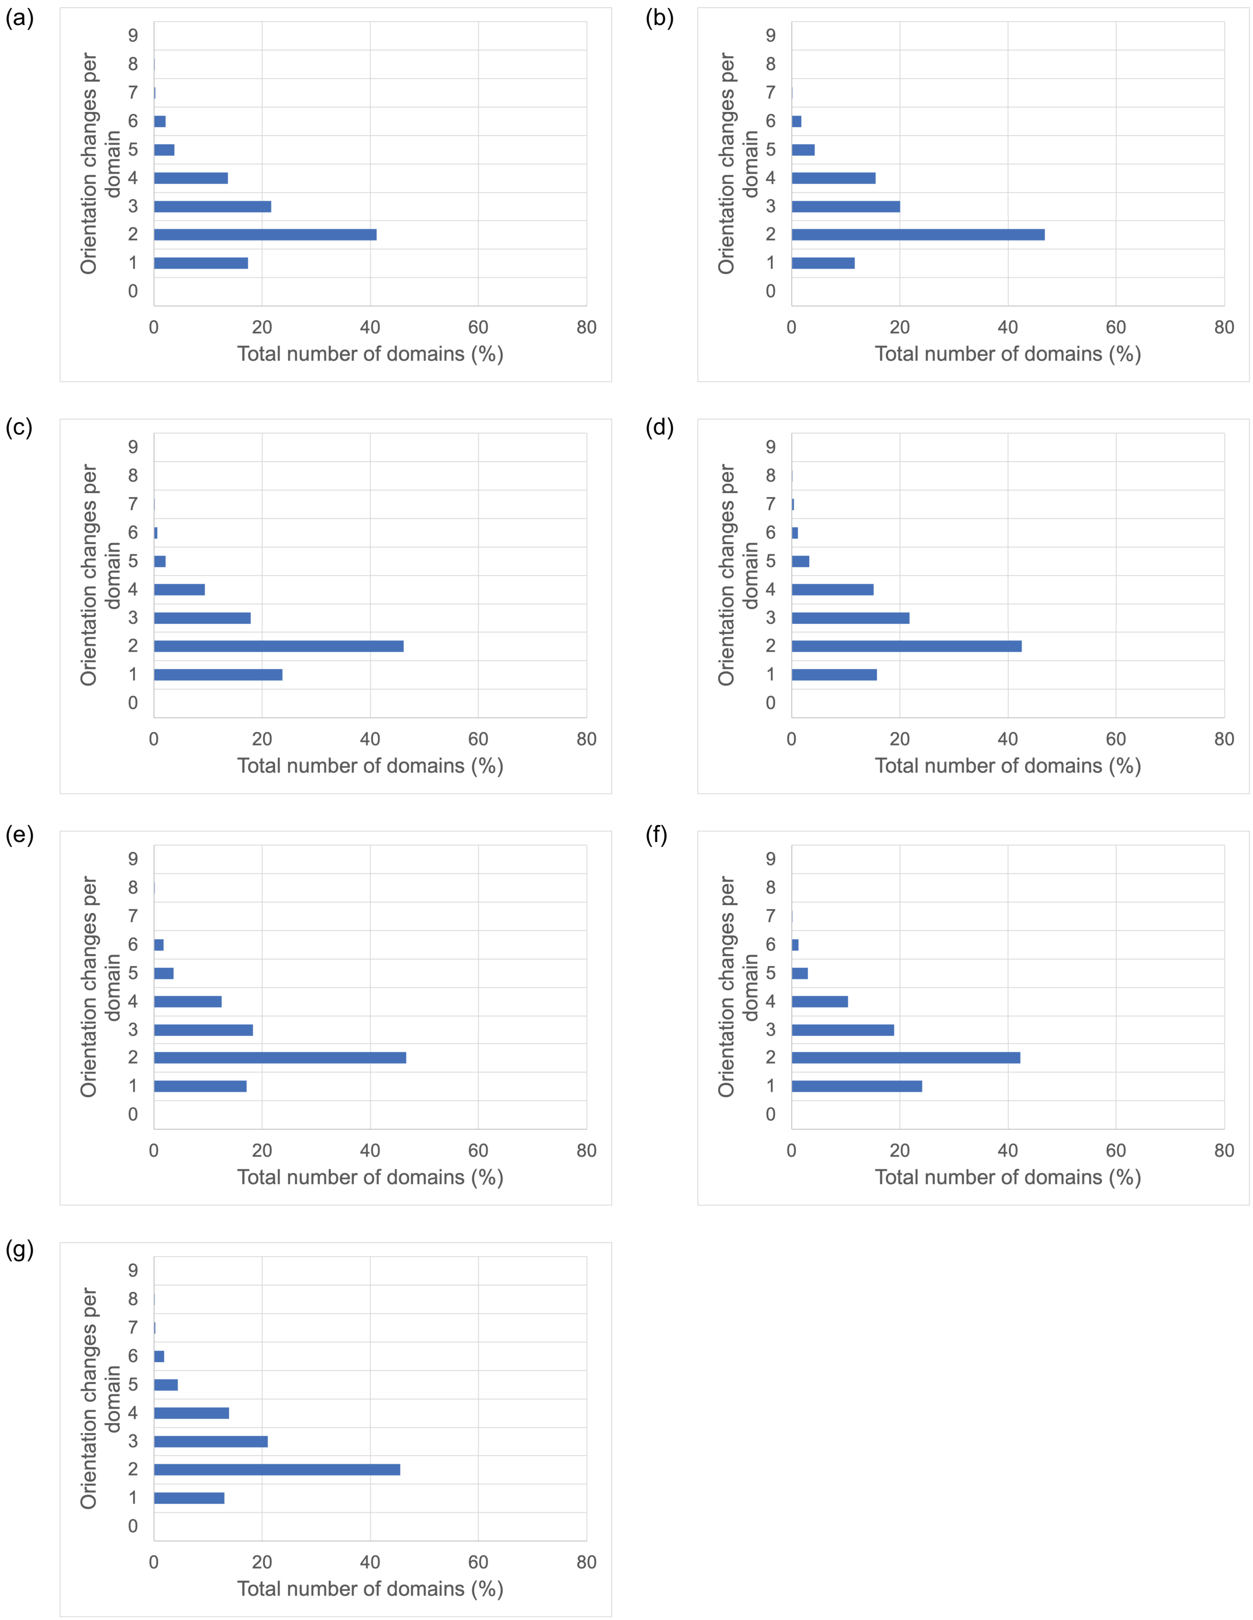


Figure S4. Statistics of polarization switching events in the dynamical simulations of multidomain $BiFeO_3$ films represented as a system of 10 domains (2 at the ends are frozen and 8 in the middle are allowed to evolve) obtained using the parameter sets presented in Table II of the main text. The histograms show the number of domains that switched in a certain number of steps in 100 runs. Panels (a) to (g) correspond to the parameter sets (i) to (vii) presented in Table II of the main text.

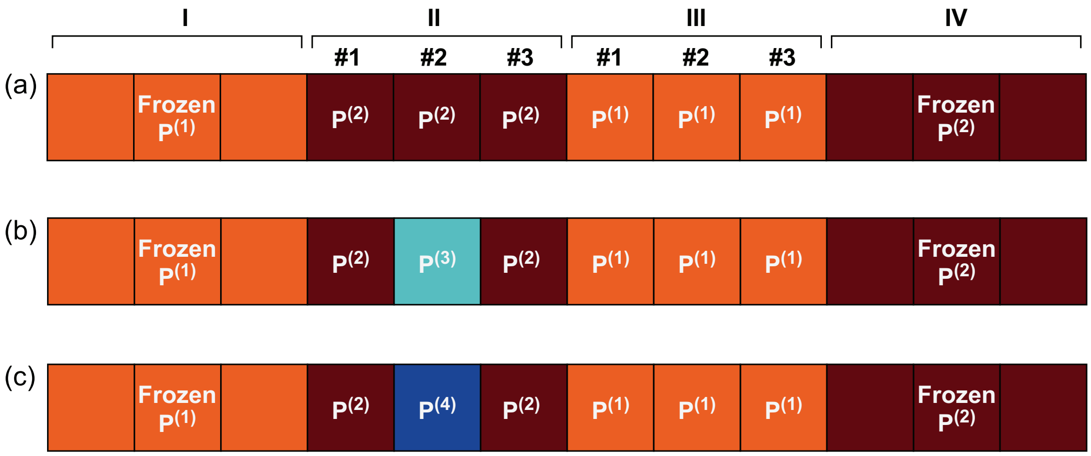


Figure S5. Approximation of multidomain $BiFeO_3$ thin film as a series of large domains each of which consists of three standard domains with uniform polarization $\mathbf{P}_i$, octahedral tilts $\mathbf{R}_i$ and strain $\boldsymbol{\eta}_i$. Panel (a) reflects the initial domain pattern of $BiFeO_3$ film before switching (see the sketch in Fig. 1(a) of the main text); panels (b) and (c) show the states in which the region of the sample is pre-switched (similar to the experimentally observed state shown in Fig. 1(b) of the main text).

## SIV. MODEL FOR THE SYSTEM OF DOMAINS WITH AN INTERNAL STRUCTURE

In order to be able to reproduce $71x$ polarization rotations being the first switching events in $BiFeO_3$ films, we simulate these films as one-dimensional series of large domains each having an internal structure. Namely, we consider large domains as consisting of three standard domains with uniform $\mathbf{P}_i$, $\mathbf{R}_i$ and $\boldsymbol{\eta}_i$ as shown in Fig. S5. To take into account the increased size of the domains in the model, we re-write $F_{sub}$ term (Eq. (16) of the main text) as follows:

$$\begin{aligned} F_{sub} =& \frac{1}{2} K_{elas,xy} \sum_{j=1}^{N-1} (\eta_{j(1),xy} + \eta_{j(2),xy} + \eta_{j(3),xy} + \\ & \eta_{j+1(1),xy} + \eta_{j+1(2),xy} + \eta_{j+1(3),xy})^2, \end{aligned} \tag{S7}$$

where (1), (2) or (3) indicate small domains inside the large domains $j$, and $N$ is the total number of large domains. We employ the system of 4 large domains (we indicate them as I, II, III and IV), two of which are frozen (I and IV) and consider three starting configurations shown in Fig. S5: (i) corresponds to the experimentally reported initial domain configuration of $BiFeO_3$ film shown in Fig. 1(a) of the main text; (ii) and (iii) represent the sample in which a certain area is pre-switched (see Figs. 1(b) of the main text) by 109° or 180°, respectively, while the rest of the sample remains in the initial state. We use the parameter sets presented in Table II of the main text, and for each set we perform 50 simulations in which we let the system to evolve in time at T=300 K with no applied electric field. We analyze the number (in % among 50 runs) of $71x$ $\mathbf{P}$ rotations. We expect more of these switching events to occur in the vicinity of pre-switched domains in configuration (ii) and (iii), since they would occur to minimize the elastic energy penalties as well as those due to structural discontinuity at the domain walls (Eq. (12) of the main text). In configuration (i), in turn, $71x$ $\mathbf{P}$ switches would occur due to thermal fluctuations. However, we could not see a clear trend in these numbers and make definitive conclusions. This can originate from the approach that we use to treat large domains. For example, by Eq. S7 we impose that the sum of $\eta_{xy}$ in the neighboring large domains equals to zero as enforced by a $DyScO_3$ substrate. In the state (ii) (see Fig. S5(b)), the pre-switched unit II,2 has $\eta_{xy} < 0$ which is unfavorable (domains II,1 and II,3 have $\eta_{xy} > 0$, and all domains inside the large domain III have $\eta_{xy} < 0$). This can be compensated by $P_x$ reversal in the domain II,2 (resulting in $\mathbf{P}^{(4)}$ orientation). However, as one can see from the Eq. S7, $F_{sub}$ can be also minimized by $71x$ switch in any of the small domains inside the large domain III, which complicates the analysis. Therefore, we conclude that our approach cannot describe $71x$ $\mathbf{P}$ rotations as the first switching events, and one rather have to employ more complex approaches such as, for example, phase-field methods.

---

* natalya.fedorova@list.lu

[†] jorge.iniguez@list.lu

[1] O. Diéguez, P. Aguado-Puente, J. Junquera, and J. Íñiguez, Phys. Rev. B **87**, 024102 (2013).
[2] N. S. Fedorova, D. E. Nikonov, H. Li, I. A. Young, and J. Íñiguez, Phys. Rev. B **106**, 165122 (2022).
